# Supplementary material for: Dressed-state Hamiltonian engineering in a strongly interacting solid-state spin ensemble
Source: arXiv:2512.09043 ancillary file (2025-12-09)
Supplement: Supplementary file 1 [file SI.pdf]

## Supplementary Materials for

# Dressed-state Hamiltonian engineering in a strongly interacting solid-state spin ensemble

Haoyang Gao[1], Nathaniel T. Leitao[1], Siddharth Dandavate[1], Lillian B. Hughes Wyatt[2,3], Piotr Put[1], Mathew Mammen[4], Leigh S. Martin[1], Hongkun Park[1,5], Ania C. Bleszynski Jayich[6], Mikhail D. Lukin[1,†]
[†]To whom correspondence should be addressed;
E-mail: lukin@physics.harvard.edu
(Dated: December 5, 2025)

### CONTENTS

I. Experimental Methods 2
I.1. Diamond Sample 2
I.2. Experimental Circuits 2
I.3. Field Alignment Procedure 3
I.4. $T_2^*$ and $T_{2,\mathrm{Hahn}}$ Characterizations 4
I.5. Floquet Engineering Pulse Sequences 4
I.6. Derivation of Modified Disorder-order Protocol 6

II. Data Analysis Details 8
II.1. Disorder-order Measurements 8
II.1.1. Data Normalization 8
II.1.2. Time-dependent Qubit Frequency 8
II.2. Sensing Experiments: Benefits and Overheads 8

III. Full Derivation of the Effective Interaction 10

IV. Generalization to Other Higher Spin Systems 11

References 12

# I. EXPERIMENTAL METHODS

## I.1. Diamond Sample

The diamond sample used in this work is the same bulk sample used in Ref. [1].

Diamond homoepitaxial growth and nitrogen doping were performed via plasma-enhanced chemical vapor deposition (PECVD) using a SEKI SDS6300 reactor on a (100) oriented electronic grade diamond substrate (Element Six Ltd.). Prior to growth, the substrate was fine-polished by Syntek Ltd. to a surface roughness of ~200-300 pm, followed by a 4-5 $\mu$m etch to relieve polishing-induced strain. The growth conditions consisted of a 750 W plasma containing 0.5% $^{12}CH_4$ in 400 sccm $H_2$ flow held at 25 torr and ~730 °C according to a pyrometer. A 125 nm-thick isotopically purified (99.998% $^{12}$C) buffer layer was grown, followed by a 185 nm-thick $^{15}$N-doped layer (1 sccm $^{15}N_2$ gas), and a 100 nm-thick $^{12}C$ capping layer. After growth, the sample was characterized with secondary ion mass spectrometry (SIMS) to estimate the isotopic purity and epilayer thickness.

The diamond was further electron irradiated and annealed to generate enhanced NV center concentrations. Irradiation was performed with the 200 keV electrons of a transmission electron microscope (TEM, ThermoFisher Talos F200X G2 TEM). The irradiation time was varied to create spots that range in dose from $10^{17}$-$10^{21}$ e$^-$/cm$^2$, and the reported experiments are performed at one spot with irradiation dose $2.4 \times 10^{19}$ e$^-$/cm$^2$. The sample then underwent subsequent annealing at $850°$ C for 6 hours in an Ar/$H_2$ atmosphere, during which the vacancies diffuse and form NV centers. After irradiation and annealing, the sample was cleaned in a boiling triacid solution (1:1:1 $H_2SO_4$:$HNO_3$:$HClO_4$) and annealed in air at $450°$ C to oxygen terminate the surface and help stabilize the negative NV$^-$ charge state for further measurements.

The density of NV centers in the confocal spot is estimated based on XY16 decay timescale measured in the on-axis field configuration. Due to the slight inhomogeneity of the sample, and the fact that the one- and two-groups experiments are performed on different coplanar waveguides (CPW, see Fig. I.1(b-c)), we independently characterized the NV density in these two cases, as it is challenging to keep the working spot exactly the same after switching the CPW. For the one-group experiments, we measured an XY16 decay timescale of 21.5 $\mu$s, corresponding to a single-group NV$^-$ density of 246 ppb. For the two-groups experiments, we separately characterized the density of NV$^-$ in the two groups by aligning the magnetic field along each of them. The measured XY16 decay timescales are 20.6 $\mu$s and 19.9 $\mu$s, corresponding to NV$^-$ densities of 257 ppb and 266 ppb. The conversion between XY16 decay timescale and NV$^-$ density is obtained empirically based on numerical simulations, assuming that the decay is dominated by dipolar interaction between NV centers.

## I.2. Experimental Circuits

An overview of the experimental circuits is shown in Fig. I.1(a), where the microwave (MW), the pulsed current, and the target signal for sensing are combined and delivered via the same coplanar waveguide (CPW), on which the diamond sample is placed. Due to the different direction of $B_\perp$ in the one- and two-groups configurations (see main text Fig. 1(c)), we use different central geometries of the CPW to generate pulsed field with corresponding directions that cancels $B_\perp$ during initialization and readout. The CPW geometries for these two configurations are shown in Fig. I.1(b-c).

As a remark on the designs of the CPW geometries, we point out that there is more flexibility in the design for the one-group perpendicular field configuration (Fig. I.1(b)), because the only requirement for high quality initialization and readout is an on-axis total field during it, instead of a field equal to zero. As a consequence, it is acceptable if the pulsed field direction is not exactly perpendicular to the NV axis, as long as it has a strong enough perpendicular component that overcomes $B_\perp$. However, the requirement becomes tighter for the two-groups perpendicular field configuration, because the only field that is simultaneously "on-axis" to both groups is a zero field. Therefore, $B_\perp$ has to be canceled exactly during initialization and readout, which motivated the design in Fig. I.1(c).

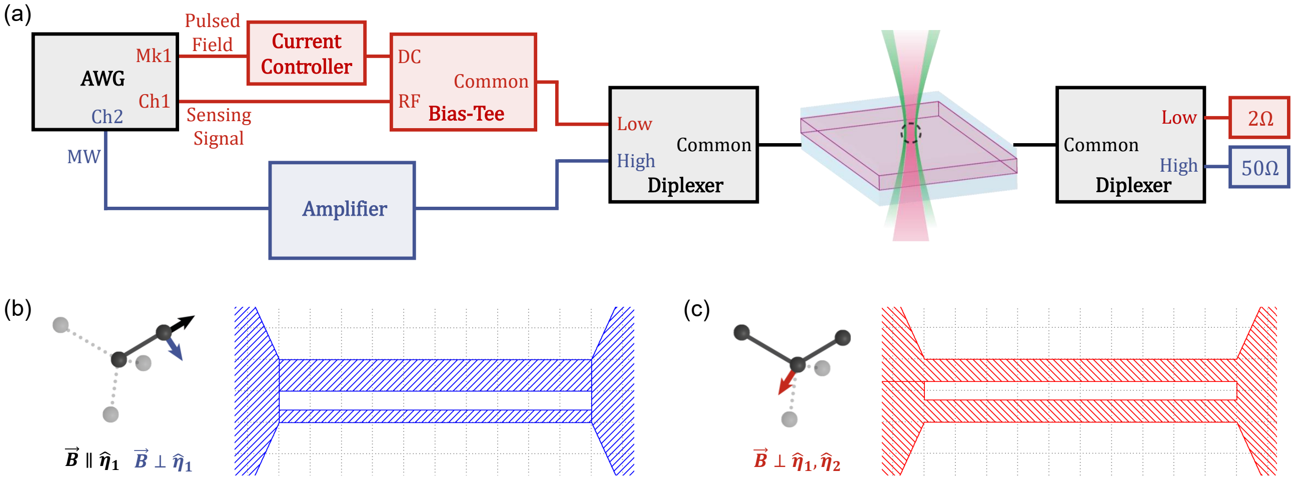


FIG. I.1: **The experimental circuits.** (a) Schematic of the whole circuit used in this work. In this diagram, components relevant to the microwave are labeled in blue, components relevant to the pulsed field or the sensing signal are labeled in red, and components common to both are labeled in gray. The 2 $\Omega$ resistor at the end of the circuit is used for monitoring the pulsed current. The circuit is conceptually the same as in Ref. [2] except the addition of the sensing signal. (b) The central feature of the coplanar waveguide used in one-group on-axis and perpendicular field configurations. The thicknesses of the two wires are 10 $\mu$m and 4 $\mu$m, and the separation between them is 6 $\mu$m. As a reference, each grid on the background represents 10 $\mu$m. The experiments are performed at a confocal spot between the two wires, where a pulsed field tilted in space is generated by the two wires with different thicknesses, which is designed to efficiently overcome $B_\perp$ during initialization and readout. (c) Same as (b), but for the two-groups perpendicular field configuration. The thicknesses of both wires are 7 $\mu$m, and the separation between them is 6 $\mu$m. The same thicknesses of the two wires are chosen to generate an in-plane pulsed field, which is required for simultaneously achieving high quality initialization and readout for the two groups.

To generate the required strength of the pulsed field that cancels $B_\perp$, a pulsed current up to 3 A is required. To prevent thermal failure of the coil, the circuit was fabricated on a diamond substrate (a separate diamond substrate that supports the NV containing diamond from below, instead of the NV containing diamond itself) with a heat conductivity three orders of magnitude better than glass. We note that this might be an overkill, given that sapphire substrate is enough for 1 A current (see Ref. [2]). Materials like silicon carbide probably provide high enough thermal conductivity, but we did not choose it due to the poor photon collection efficiency through it.

### I.3. Field Alignment Procedure

In the conventional on-axis field configuration, the field alignment is typical done by overlapping the electron-spin-resonance (ESR) peaks of the other three groups of NVs, which guarantees an on-axis field for the main group due to the symmetry of diamond lattice. However, there is no symmetry based methods for field alignment in the perpendicular field configuration, making the procedure non-trivial.

The field alignment in the one-group perpendicular field configuration is done through a feedback procedure. In this procedure, one first locate all 8 ESR peaks originated from the 4 groups of NVs, and then extract the field $\vec{B}$ relative to the diamond lattice coordinate system by fitting the frequencies of the 8 peaks. After that, one adjust the magnetic field based on its current value and target value, and repeat the process until the field is well aligned.

However, such method does not work well in the two-groups perpendicular field configuration, as there exist one direction along which the frequencies of all 8 peaks are $1^{\text{st}}$ order insensitive to the change of B-field. More specifically, if we assume that the four groups of NVs are along the directions $(1,1,1)$, $(-1,-1,1)$, $(1,-1,-1)$, and $(-1,1,-1)$, and $\vec{B} \propto (-1,1,0)$ is the perpendicular field that addresses the first two groups, the insensitive direction would be along $(1,1,0)$. To align the field precisely, we follow the following steps:

- To align the field along $(-1,1,0)$, we measure the frequency of the transition $|\tilde{0}\rangle \leftrightarrow |\tilde{B}\rangle$, which is sensitivity to the perpendicular field strength.

- To align the field along $(0,0,1)$, we overlap the lower frequency transition of the third and fourth groups (i.e. the two groups not perpendicular to $B_\perp$), which exhibits a $1^{\text{st}}$ order splitting when the field is deviated from its target value along

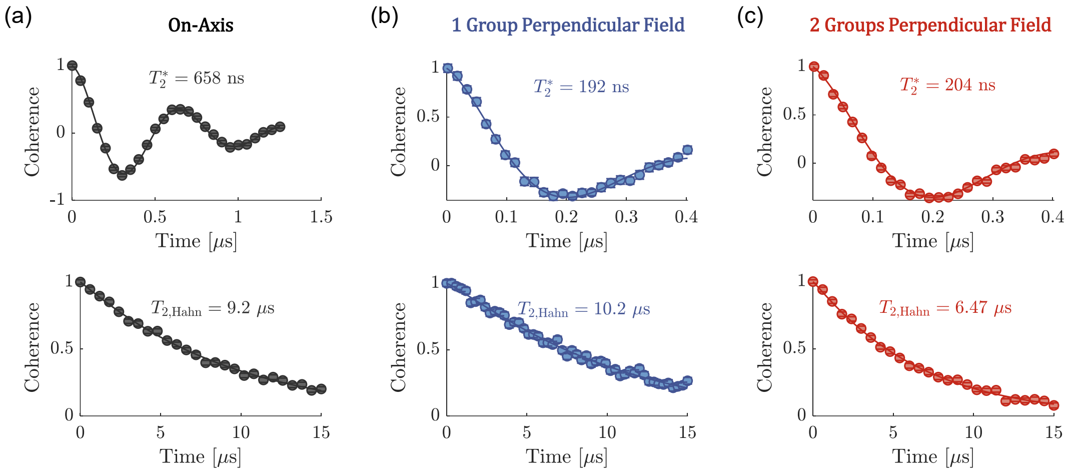


FIG. I.2: **$T_2^*$ and $T_{2,\mathrm{Hahn}}$ characterizations.** (a) The results in the on-axis field configuration. (b-c) The results in the one- and two-groups perpendicular field configuration. The data shows a much shorter $T_2^*$ but roughly the same $T_{2,\mathrm{Hahn}}$, indicating stronger but more static on-site disorder in the perpendicular field configurations.

this direction.

- To align the field along the insensitive direction $(1, 1, 0)$, we sweep the field along this direction and measure the frequencies $f_1$ and $f_2$ of the transitions $|\tilde{0}\rangle \leftrightarrow |D\rangle$ and $|\tilde{0}\rangle \leftrightarrow |\tilde{B}\rangle$ (of the two groups perpendicular to $B_\perp$). The value $2f_1 - f_2$ is expected to be maximized under exactly perpendicular field, and we rely on a second order polynomial fit to extract the location of the maximum.

- Repeat the first step again to correct for small change of the field strength introduced in the second and third steps.

### I.4. $T_2^*$ and $T_{2,\mathrm{Hahn}}$ Characterizations

We characterized $T_2^*$ and $T_2$ (under Hahn echo) in the three configurations introduced in main text Fig. 1(c), and the results are summarized in Fig. I.2. Here we see that the perpendicular field configurations exhibit a much shorter $T_2^*$ but roughly the same $T_{2,\mathrm{Hahn}}$. This indicates a stronger but more static on-site disorder, which is beneficial for disorder-order type measurements[3], as shown in main text Fig. 4(c). The stronger on-site disorder may originate from strain inhomogeneity, as the $\{|\tilde{0}\rangle, |\tilde{B}\rangle\}$ encoding is sensitive to it[4].

### I.5. Floquet Engineering Pulse Sequences

In this work, we use three different Floquet engineering (and dynamical decoupling) pulse sequences:

- The "cXY8" pulse sequence (Fig. I.3) - standing for "concatenated XY8" - is used to decouple on-site disorder in all experiments in perpendicular field configurations. We choose this sequence for its improved robustness against coherent pulse errors compared to XY8[5] (Fig. I.5(a)). Such robustness comes from the concatenated structure of the sequence, which guarantees that accumulated coherent errors in the inner XY8 are coherently canceled by the outer XY8. We note that the necessity of such concatenated sequences originates from the short $T_2^*$ in the perpendicular field configuration (Fig. I.2), which requires fast decoupling (one pulse every 50 ns) that leads to a total pulse number exceeding 6000 within the coherence time of the system. The sensing experiment in the on-axis field configuration (main text Fig. 3) also used cXY8 for consistency, although it is not necessary.

- The "DROID-60" pulse sequence[9] is used in the sensing experiment (main text Fig. 3), as an established pulse sequence commonly used in sensing applications. Although there exist a higher-order sensing sequence "DIRAC2"[10] that has shown better sensitivity than DROID-60, it is more suitable for target signals with lower frequencies due to its special way of synchronization with the signal. For the 10 MHz target signal used in this work, DIRAC2 would not perform well

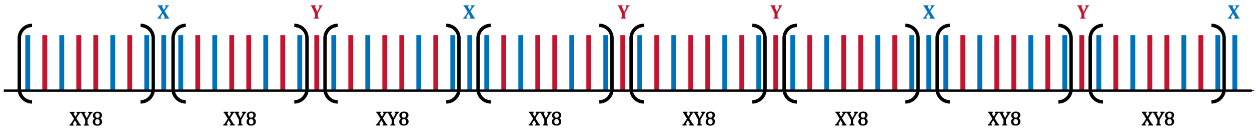


FIG. I.3: **The pulse sequence “cXY8”.** The pulse sequence cXY8 is a concatenation of XY8 with itself. The outer XY8 cancels residual coherent pulse errors in the inner XY8, improving the robustness of the pulse sequence. The blue (red) rectangles represent $\pi$-pulses around X (Y).

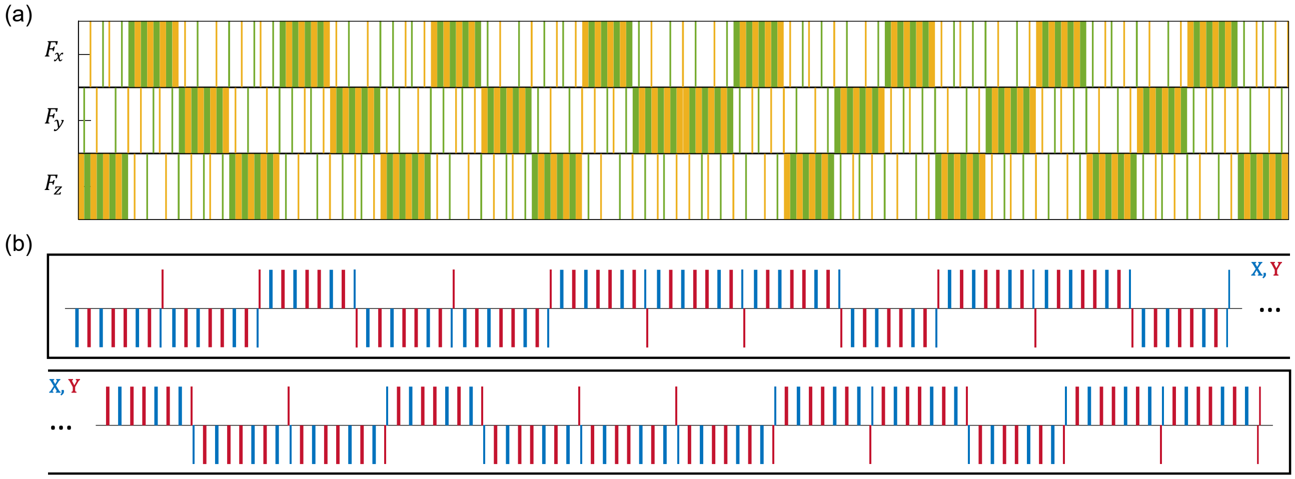


FIG. I.4: **The pulse sequence “cXY8-DROID-vXY4-Mirror”.** (a) Frame representation[6] of the pulse sequence, showing the concatenated structures discussed in Section. I.5. (b) The actual pulses constituting this sequence. The thin lines represent $\pi/2$-pulses and the thick lines represent $\pi$-pulses. The color of the pulses represent the pulse axis (X or Y), and the direction of them (up or down) represent the two opposite rotation directions (e.g. $+\pi/2$ pulse and $-\pi/2$ pulse). The ellipsis in the plot indicates that the two rows are connected. The plot is a conceptual illustration of the pulse sequence and is not drawn in proportion to the actual time duration. The actual pulse sequence applied in the experiment uses cosine envelop with $\pi$-pulse duration $t_\pi = 40$ ns and pulse spacing $\tau = 10$ ns.

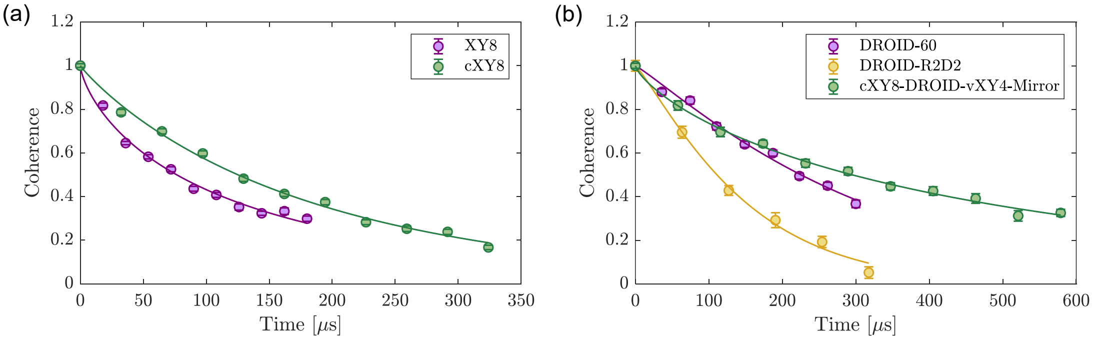


FIG. I.5: **Pulse sequence comparisons.** (a) Comparison of the decay of an initial state polarized along X, under the pulse sequences XY8[7] and cXY8 (i.e. concatenate[5] XY8 with itself). The interaction is tuned to the native SU (2) point in the two-groups perpendicular field configuration. (b) Similar comparison in the on-axis field configuration with Floquet engineered SU (2) symmetry. The pulse sequences are DROID-60[6], DROID-R2D2[8], and cXY8-DROID-vXY4-Mirror (used in this work).

because it requires a very high pulse rate (one pulse per 25 ns) to synchronize with the signal, which would lead to fast accumulation of pulse errors.

- The pulse sequence we call "cXY8-DROID-vXY4-Mirror" (Fig. I.4) is used for Floquet engineering of various XXZ Hamiltonian[3] in the on-axis field configuration (main text Fig. 2). This sequence can be viewed as an improved version of the higher-order decoupling sequence "DROID-R2D2" introduced in[8], suitable for lower density NV ensembles that have long enough coherence time for such a long pulse sequence. The name of this pulse sequence stands for its structure, which involves the concatenation of the following four layers:

  – The inner layer is an XY8, targeting at robust disorder decoupling on fastest possible timescale.

  – The second layer is the DROID[6] or WAHUHA[11] structure that symmetrizes the dipolar interaction into $\mathrm{SU}(2)$ symmetry.

  – The third layer can be viewed as further concatenation with XY4 using virtual pulses[12], serving the role of canceling coherent pulse errors accumulated in the first two layers. We note that such concatenation with XY4 automatically guarantees the satisfaction of all design rules for higher order dynamical decoupling[8].

  – The outer layer is a mirror symmetrization (in term of the frame representation in Fig. I.4(a)) that we found helpful experimentally. We note that previous DROID-type sequences[6, 8] also have the same or similar structures.

  This sequence is our current best in term of coherence time of the NV ensemble used in this work (Fig. I.5(b)), representing the state-of-the-art Floquet engineering. We note that although this sequence offers a coherence time longer than that of DROID-60, it cannot be used for sensing applications because the toggling frames are not synchronized to the target signal[9].

The timing of the pulse sequences are chosen as follow: all pulse sequences use $\pi$-pulse duration $t_\pi = 40$ ns and pulse spacing $\tau = 10$ ns. The pulse wavepacket is chosen as cosine pulse (i.e. the oscillation amplitude $A(t) \propto \left(1 - \cos\frac{2\pi t}{t_\pi}\right)$, for $t \in (0, t_\pi)$) to reduce the off-resonant $|\tilde{0}\rangle \leftrightarrow |D\rangle$ transition, which contributes to leakage out of the qubit subspace $\{|\tilde{0}\rangle, |\tilde{B}\rangle\}$. Effects of finite pulse duration[6] are considered in the calculation of the XXZ parameter $\lambda$ in main text Fig. 2(d).

Finally, we note that subsampling technique[3] is used for measuring the red data points in main text Fig. 2(c), in order to include more data points within the relatively short decay timescale.

### I.6. Derivation of Modified Disorder-order Protocol

In the modified disorder-order protocol in main text Fig. 4(b), the disorder winding time is chosen as $\tau_{\mathrm{wind}} \sim 3.5T_2^\star$ to ensure that each spin is initially polarized along a random direction, as required for measuring infinite temperature auto-correlators. In addition, the dephasing time is chosen as $\tau' = 3\tau_{\mathrm{wind}}$. In this section, we present a detailed derivation connecting such protocol to the local auto-correlator $C_{\mathrm{Local}}^{ZZ}$, and explain the timing choice above.

Generically, the modified disorder-order protocol in main text Fig. 4(b) results in a final state

$$|\psi_{\theta,\phi}\rangle = V_\theta^\dagger U(t) W_\phi V_\theta |+\rangle^{\otimes N}, \tag{I.1}$$

where $U(t)$ is the many-body evolution, and

$$\begin{aligned} V_\theta &\equiv \prod_j \exp(-i\theta_j Z_j/2) \\ W_\phi &\equiv \prod_j \exp(-i\phi_j X_j/2) \end{aligned} \tag{I.2}$$

are the evolution during disorder winding and dephasing steps, with $\theta_j$ and $\phi_j$ being the rotation angle of the $j^{\mathrm{th}}$ spin under the local disorder field. For simplicity, we have done a frame transformation under the $\frac{\pi}{2}$-pulses that rotate $X \leftrightarrow Z$ (see main text Fig. 4(b)), which leads to the rotation around X in $W_\phi$.

In this state, the global measurement along X-axis yields the signal

$$
\begin{aligned}
S(t) &= \sum_i \int_{\theta,\phi} \mathrm{Tr}\left[X_i V_\theta^\dagger U(t) W_\phi V_\theta |+\rangle^{\otimes N} \langle +|^{\otimes N} V_\theta^\dagger W_\phi^\dagger U^\dagger(t) V_\theta\right] \\
&= \sum_i \int_{\theta,\phi} \mathrm{Tr}\left[\left(U^\dagger(t) V_\theta X_i V_\theta^\dagger U(t)\right)\left(W_\phi V_\theta |+\rangle^{\otimes N} \langle +|^{\otimes N} V_\theta^\dagger W_\phi^\dagger\right)\right] \\
&= \sum_i \int_{\theta,\phi} \mathrm{Tr}\left[\left(\cos\theta_i X_i(t) + \sin\theta_i Y_i(t)\right)\prod_j \frac{1+\cos\theta_j X_j + \sin\theta_j\cos\phi_j Y_j + \sin\theta_j \sin\phi_j Z_j}{2}\right] \\
&\equiv \sum_i C_i(t),
\end{aligned}
\tag{I.3}
$$

where

$$
C_i(t) = \sum_\chi f_i(\chi)\,\mathrm{Tr}\left[X_i(t)\chi\right] + g_i(\chi)\,\mathrm{Tr}\left[Y_i(t)\chi\right] \tag{I.4}
$$

denotes a sum over Pauli strings $\chi = \sigma_1^{\mu_1} \otimes \sigma_2^{\mu_2} \otimes \ldots \otimes \sigma_N^{\mu_N}$. The coefficients read

$$
\begin{aligned}
f_i(\chi) &= \int_{\theta,\phi} \cos\theta_i \prod_j a_{\mu_j}(\theta_j,\phi_j) \\
g_i(\chi) &= \int_{\theta,\phi} \sin\theta_i \prod_j a_{\mu_j}(\theta_j,\phi_j),
\end{aligned}
\tag{I.5}
$$

where

$$
a_\mu(\theta,\phi) = (1, \cos\theta, \sin\theta\cos\phi, \sin\theta\sin\phi) \tag{I.6}
$$

is the decomposition of the second term of Eq. (I.3) in Pauli basis.

Now we consider two scenarios for the joint distribution of $(\theta,\phi)$. The first scenario is an idealized case, where $\theta$ and $\phi$ are independent variables uniformly distribution between 0 and $2\pi$. In this scenario, Eq. (I.5) simplifies to

$$
f_i(\chi) = \delta(\chi, X_i)/2, \quad g_i(\chi) = 0, \tag{I.7}
$$

since all integrals in Eq. (I.5) are decoupled. As a direction consequence, the signal we measure is

$$
S(t) = \frac{1}{2}\sum_i \mathrm{Tr}\left[X_i(t) X_i\right]. \tag{I.8}
$$

This expression is proportional to the local auto-correlator $C^{ZZ}_{\mathrm{Local}}$, up to a $X \leftrightarrow Z$ rotation arising from the frame transformation introduced at the beginning of the derivation.

The second scenario is an experimentally motivated scenario, building upon the observation that both $\theta_i$ and $\phi_i$ originates from the on-site disorder of the same spin. Therefore, a better description of the measurement protocol is that $\phi_i$ and $\theta_i$ are constraint by $\phi_i = r\theta_i$, where $r = \frac{\tau'}{\tau_{\mathrm{wind}}}$ is the ratio of the dephasing time and disorder winding time. We still assume independent sampling of $\theta_i$ across different sites, as there is no clear evidence against it. In this scenario, the functions $f$ and $g$ are slightly more complicated:

$$
\begin{aligned}
f_i(\chi) &= \left(\int_{-\pi}^{\pi} \frac{\mathrm{d}\theta_i}{2\pi}\cos\theta_i a_{\mu_i}(\theta_i, r\theta_i)\right)\prod_{j\neq i}\left(\int_{-\pi}^{\pi}\frac{\mathrm{d}\theta_j}{2\pi} a_{\mu_j}(\theta_j, r\theta_j)\right) \\
g_i(\chi) &= \left(\int_{-\pi}^{\pi} \frac{\mathrm{d}\theta_i}{2\pi}\sin\theta_i a_{\mu_i}(\theta_i, r\theta_i)\right)\prod_{j\neq i}\left(\int_{-\pi}^{\pi}\frac{\mathrm{d}\theta_j}{2\pi} a_{\mu_j}(\theta_j, r\theta_j)\right).
\end{aligned}
\tag{I.9}
$$

It is straightforward now to evaluate the single site integrals:

$$
\begin{aligned}
\int_{-\pi}^{\pi}\frac{\mathrm{d}\theta}{2\pi} a_\mu(\theta, r\theta) &= \left(1, 0, 0, \frac{\sin\pi r}{\pi(1-r^2)}\right)_\mu \\
\int_{-\pi}^{\pi}\frac{\mathrm{d}\theta}{2\pi}\cos\theta a_\mu(\theta, r\theta) &= \left(0, \frac{1}{2}, 0, -\frac{\sin\pi r}{\pi(4-r^2)}\right)_\mu \\
\int_{-\pi}^{\pi}\frac{\mathrm{d}\theta}{2\pi}\sin\theta a_\mu(\theta, r\theta) &= \left(0, 0, \frac{2\sin\pi r}{\pi r(4-r^2)}, 0\right)_\mu.
\end{aligned}
\tag{I.10}
$$

Here we see that for any $r \in \mathbb{Z},\ r \geq 3$, the functions $f$ and $g$ simplify to Eq. (I.7) and thus lead to a clean experimental signal Eq. (I.8). For simplicity, we chose the smallest option $r = 3$ in our experiments.

# II. DATA ANALYSIS DETAILS

## II.1. Disorder-order Measurements

### *II.1.1. Data Normalization*

In addition to the intrinsic dynamics under dipolar coupling, there are two extrinsic decay sources affecting the data in the disorder-order measurements[3]:

- As shown in main text Fig. 4(c), one source of extrinsic decay is non-ideal unwinding, as the on-site disorder is not completely static between the winding and unwinding steps. We denote such decay as $C_{\mathrm{Unwinding}}(t)$.
- Another source of extrinsic decay is decoherence during the decoupling pulse sequence, which can be estimated from the measured decay of an initial state polarized along +Z (while applying the decoupling sequence). We emphasize that the measured decay is much faster than bare $T_1$ of the system, because the decoupling sequence applies non-trivial rotations to the initial state and thereby disturbs its dynamics. As a result, such decay is not double counted in the measurement of $C_{\mathrm{Unwinding}}(t)$, where no decoupling sequence is applied. We denote such decay as $C_{\mathrm{Global}}(t)$.

In the reported data in main text Fig. 2(c), the contribution from the first source is normalized out according to

$$C_{\mathrm{Normalized}}(t) \equiv \frac{C_{\mathrm{Raw}}(t)}{C_{\mathrm{Unwinding}}(t)}, \tag{II.1}$$

but the contribution from the second source is not normalized out. This choice is made to keep consistency with the global decay measurements (i.e. the semi-transparent circle markers) that are not normalized by themselves. In the end, such choice does not affect the data strongly, as the global decay is much slower than the intrinsic dynamics (see main text Fig. 2(c)). The raw disorder-order data $C_{\mathrm{Raw}}(t)$ and the extrinsic decay $C_{\mathrm{Unwinding}}(t)$ behind main text Fig. 2(c) are shown in Fig. II.1.

Slightly differently, the data reported in main text Fig. 4(d) is normalized against both extrinsic decay sources, according to

$$C_{\mathrm{Normalized}}(t) \equiv \frac{C_{\mathrm{Raw}}(t)}{C_{\mathrm{Unwinding}}(t)\, C_{\mathrm{Global}}(t)}, \tag{II.2}$$

as an attempt to extract the intrinsic decay originated from spin transport. The raw data $C_{\mathrm{Raw}}(t)$ and the extrinsic decays $C_{\mathrm{Unwinding}}(t)$ and $C_{\mathrm{Global}}(t)$ are shown in Fig. II.2.

### *II.1.2. Time-dependent Qubit Frequency*

A subtlety in this work is the time-dependent qubit frequency, originated from residual tails of the pulsed field after switching it off. Such time-dependent qubit frequency leads to a systematic mismatch of the detuning during the winding and unwinding steps (see main text Fig. 4(b)), which contributes to an additional rotation of the final spin polarization around Z axis. Considering the effect of such rotation, we measure the final spin polarization along both X and Y axes ($C_{\mathrm{X}}$ and $C_{\mathrm{Y}}$), and compute the signal as

$$C = \sqrt{C_{\mathrm{X}}^2 + C_{\mathrm{Y}}^2 - (\delta C_{\mathrm{X}})^2 - (\delta C_{\mathrm{Y}})^2}, \tag{II.3}$$

where we subtract the noise $\delta C_{\mathrm{X}}$ and $\delta C_{\mathrm{Y}}$ (estimated from the errorbar), which tends to artificially increase $C$. The measurement of $C_{\mathrm{Unwinding}}(t)$ mentioned in Section. II.1.1 is also affected by this rotation, and the data is processed in the same way, before performing the normalization.

## II.2. Sensing Experiments: Benefits and Overheads

In this section, we analyze the benefits and overheads of the two-groups perpendicular field configuration in the sensing experiments (main text Fig. 3), in comparison to the on-axis field configuration with DROID-60. As discussed in main text Fig. 3(a), the ideal-case benefits include:

- Doubled contrast, leading to 2x enhancement of the sensitivity.
- Avoiding the $\sqrt{3}$ reduction of effective field in DROID, leading to $\sqrt{3}$x enhancement.

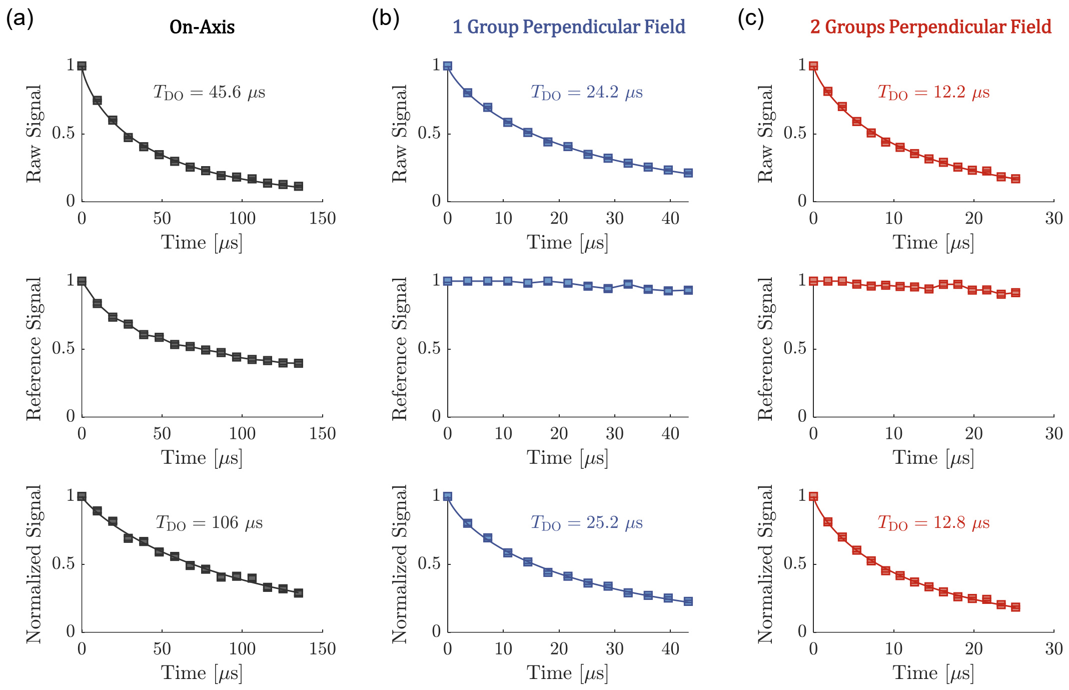


FIG. II.1: **Disorder-order data normalization.** (a) The data normalization behind main text Fig. 2(c), in the on-axis field configuration. The first row is the raw disorder-order decay data, and the second row is the measured reference decay due to imperfect disorder unwinding. Dividing the raw data by the reference signal point-by-point leads to the third row, which is reported in main text Fig. 2(c). The curves are stretched exponential fit, and the fitted $1/e$ decay timescales are labeled next to the data. Here we see a significant decay of the reference signal, which has a strong effect on the observed decay timescale. (b-c) Same as (a), but for the one- and two-groups perpendicular field configurations. The reference decay is much slower in these two configurations, and the observed decay timescale is not strongly affected by it.

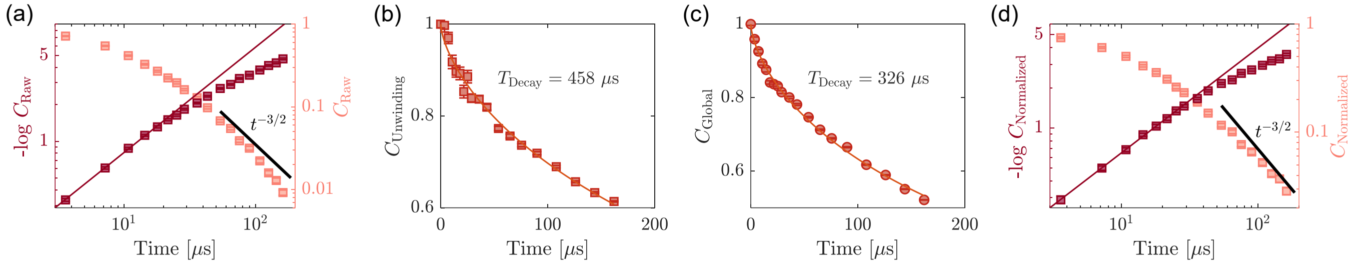


FIG. II.2: **Modified disorder-order data normalization.** (a) Raw data behind main text Fig. 4(d). (b) Measured extrinsic decay due to imperfect unwinding, as discussed in Section. II.1.1. The data is the same as the red data points in main text Fig. 4(c), repeated here for convenience. The curve is a stretched exponential fit, and the fitted $1/e$ decay timescale is labeled next to the data. (c) Measured extrinsic decay due to decoherence during the decoupling pulse sequence. (d) The normalized data, computed according to Eq. (II.2). The data is the same as main text Fig. 4(d), repeated here for convenience.

- 1.15 times larger magnetic moment, leading to 1.15x enhancement.

In total, these factors contributes to an ideal-case sensitivity enhancement of 4x (i.e. 12.0 dB). The relevant overheads in the two-groups perpendicular field configuration include:

- The experimentally observed contrast enhancement is not 2x, but closer to 1.8x. Possible reasons for this contrast loss include imperfections in the pulsed field alignment, loss of spin polarization during the switching of the pulsed field, and stronger background fluorescence from the other two groups of NV centers (because readout in the two-groups perpendicular field configuration is done under zero-field, where all 4 groups are "on-axis" and therefore emit more photons; see

| | Benefits | Overheads |
|---|---|---|
| Doubled contrast | 2x | |
| Avoiding DROID | $\sqrt{3}$x | |
| Larger magnetic moment | 1.15x | |
| Shorter coherence time | | 0.76x |
| Contrast loss | | 0.90x |
| Time overhead | | 0.92x |
| Total | 4x | 0.63x |

TABLE I: **Benefits and overheads for two-groups perpendicular field sensing.** This table summarizes the benefits and overheads for sensing in the two-groups perpendicular field configuration, compared to the on-axis field configuration with DROID-60 pulse sequence.

Section. I.2 for discussions). This leads to an overhead of 0.9x for the achievable sensitivity.

- The coherence time measured in absolute unit is shorter in the two-group perpendicular field configuration (180 $\mu$s), compared to DROID-60 in the on-axis field configuration (313 $\mu$s). This leads to a sensitivity overhead of $\sqrt{180/313} = 0.76$.

- It takes 20 $\mu$s after switching off the pulsed field for stabilization of the qubit frequency, which is affected by the residual tail of the pulsed field. Combined with a laser repolarization time (and other waiting time) of 20 $\mu$s, this leads to a total time overhead of 40 $\mu$s, increasing the experimental cycle from the optimal phase accumulation time 120 $\mu$s (see main text Fig. 3(c)) to 160 $\mu$s. Such overhead reduces the sensitivity in the two-group perpendicular field configuration by a factor of $\sqrt{120/160} = 0.87$. Similarly, DROID-60 in the on-axis field configuration is also affected by the laser repolarization time of 20 $\mu$s, increasing the experimental cycle from 160 $\mu$s to 180 $\mu$s, and leading to a reduction of sensitivity by a factor of $\sqrt{160/180} = 0.94$. In comparison, the time overhead leads to an additional sensitivity reduction of $0.87/0.94 = 0.92$ for the two-groups perpendicular field configuration.

Multiplying these factors together, the total sensitivity overhead in the two-groups perpendicular field case is 0.63x, and the expected sensitivity gain is therefore $4 \cdot 0.63 = 2.52$x, in consistency with the observed value of 2.6x (main text Fig. 3(c)). This analysis of benefits and overheads is summarized in Table. I.

## III. FULL DERIVATION OF THE EFFECTIVE INTERACTION

In this section, we derive the effective interaction in the perpendicular field configuration (Eq. (5-6) in the main text), starting from the original form of the dipolar Hamiltonian

$$H_{ij}^{\text{Dipole}} = -\frac{J_{\text{Dipole}}}{r^3}\left[3\left(\vec{J}_i \cdot \hat{r}\right)\left(\vec{J}_j \cdot \hat{r}\right) - \vec{J}_i \cdot \vec{J}_j\right]. \tag{III.1}$$

As discussed in the main text, the effective interaction can be obtained by projecting Eq. (III.1) onto the qubit subspace spanned by $\left\{\left|\tilde{0}\right\rangle, \left|\tilde{B}\right\rangle\right\}$, where a significant simplification comes from the observation that both $J^y$ and $J^z$ project to zero

$$\mathcal{P}\left(J^y\right) = \mathcal{P}\left(J^z\right) = 0. \tag{III.2}$$

As a consequence, the effective Hamiltonian only involves the projection of $J^x$

$$H_{ij}^{\text{eff}} = -\frac{2J_{\text{Dipole}}}{r^3} A_{\hat{x}}\left(\hat{r}\right) \mathcal{P}\left(J_i^x\right) \mathcal{P}\left(J_j^x\right), \tag{III.3}$$

where $A_{\hat{x}}\left(\hat{r}\right) \equiv \frac{3(\hat{x}\cdot\hat{r})^2 - 1}{2}$ is the dipolar anisotropy. The projection $\mathcal{P}\left(J^x\right)$ can be calculated via its matrix elements

$$\begin{aligned} \left\langle\tilde{0}\right| J^x \left|\tilde{0}\right\rangle &= -\sin\alpha \\ \left\langle\tilde{B}\right| J^x \left|\tilde{B}\right\rangle &= \sin\alpha \\ \left\langle\tilde{0}\right| J^x \left|\tilde{B}\right\rangle = \left\langle\tilde{B}\right| J^x \left|\tilde{0}\right\rangle^* &= \cos\alpha, \end{aligned} \tag{III.4}$$

where $\alpha = \tan^{-1}\left(\frac{2\gamma B_\perp}{D}\right)$ is the mixing angle of the dressed-states, as discussed in main text Eq. (2). Introducing the effective spin-$\frac{1}{2}$ operators $s^{x,y,z}$ defined in the qubit subspace, Eq. (III.4) can be written in a compact form

$$\mathcal{P}\left(J^x\right) = -\left(2\sin\alpha\right)s^z + \left(2\cos\alpha\right)s^x, \tag{III.5}$$

where the factor of 2 comes from the factor of $\frac{1}{2}$ in the definitions of $s^{x,y,z}$. Plugging Eq. (III.5) into Eq. (III.3) leads to the effective interaction

$$H_{ij}^{\text{eff}} = -\frac{J_{\text{Dipole}}}{r^3}A_{\hat{x}}\left(\hat{r}\right)\left[\left(8\cos^2\alpha\right)s_i^x s_j^x + \left(8\sin^2\alpha\right)s_i^z s_j^z - \left(8\sin\alpha\cos\alpha\right)\left(s_i^x s_j^z + s_i^z s_j^x\right)\right]. \tag{III.6}$$

Finally, applying secular approximation[13] to Eq. (III.6) cancels the term $s_i^x s_j^z + s_i^z s_j^x$, which does not conserve the energy. Similarly, the term $s_i^x s_j^x$ is transformed into $\left(s_i^x s_j^x + s_i^y s_j^y\right)/2$, leading to the final expression

$$H_{ij}^{\text{eff}} = -\frac{J_{\text{Dipole}}}{r^3}A_{\hat{x}}\left(\hat{r}\right)\left[\left(4\cos^2\alpha\right)\left(s_i^x s_j^x + s_i^y s_j^y\right) + \left(8\sin^2\alpha\right)s_i^z s_j^z\right]. \tag{III.7}$$

## IV. GENERALIZATION TO OTHER HIGHER SPIN SYSTEMS

The presented perpendicular field techniques for direct tuning of the native dipolar interaction are expected to generalize beyond NV centers, and apply to any higher spin ($S > \frac{1}{2}$) system with $\pm m$ degeneracy and non-zero zero-field splitting. To understand the generality of such techniques, we emphasize that all good properties we relied on in this work fundamentally originates from the following observation in the perpendicular field configuration:

$$\mathcal{P}\left(J^y\right) = \mathcal{P}\left(J^z\right) = 0 \tag{IV.1}$$

where $\mathcal{P}$ is the projection operator onto the qubit subspace $\left\{\left|\tilde{0}\right\rangle, \left|\tilde{B}\right\rangle\right\}$. Here we explain how this observation leads to the good properties point by point:

- The most important property is the tunability of the dipolar interaction via the strength of $B_\perp$. To understand such tunability, we consider the weak and strong $B_\perp$ limits. In the weak field limit, the permanent magnetic moments of the dressed-states approach zero, because the weak $B_\perp$ is insufficient to polarize the eigenstates along X, while polarization along Y and Z is precluded by Eq. (IV.1). As a result, there is no Ising coupling in this limit and the interaction is purely $s_i^x s_i^x + s_i^y s_i^y$. In the opposite strong $B_\perp$ limit, the field $B_\perp$ dominates over the zero-field splitting, and the dressed states become $\left|J^x = -1\right\rangle$ and $\left|J^x = +1\right\rangle$ (see main text Fig. 2(a)). These two states differ by $\Delta J^x = 2$, leading to forbiddened transition between them and therefore no exchange coupling. This results in a purely Ising interaction in the strong $B_\perp$ limit. Interpolation between these two limits thus leads to the generic expectation that the interaction can be tuned from the easy-plane side to the easy-axis side via increasing $B_\perp$.

- The perpendicular field configuration also helps us avoiding ESEEM effect[14], which is generically expected under an off-axis field. To understand this, we note that ESEEM effect fundamentally originates from non-commuting coupling of the nuclear spin to the external field, and to the electronic spin via hyperfine interaction. In the perpendicular field configuration, Eq. (IV.1) guarantees an electronic spin polarization along X, which generates a field on the nuclear spin that commutes with direct coupling to the external field (which is also along X).

- A property that simplifies the qubit interaction is that the Hamiltonian can be factorized into a spatial anisotropy term (i.e. $A_{\hat{B}_\perp}\left(\hat{r}\right)$ in main text Eq. (5)) and an XXZ anisotropy term (i.e. $g_{\text{XY}}\left(s_i^x s_j^x + s_i^y s_j^y\right) + g_{\text{ZZ}} s_i^z s_j^z$). Although this is the case for both the perpendicular field configuration and the on-axis field configuration, it is not generically expected under arbitrary field orientation (e.g. see Ref. [2], where the exchange and Ising parts exhibit different spatial anisotropy). In the perpendicular field configuration, this simplification comes from Eq. (IV.1), which guarantees that the qubits only interact with each other through their magnetic moments along X, dictating the unique spatial anisotropy factor that is shared by both the exchange and the Ising couplings.

- The perpendicular field configuration enables convenient operations with two groups of NV centers simultaneously, with the guarantee that the inter- and intra-group interaction having exactly the same form, and that the two groups having exactly the same coupling to MW drivings. As discussed in main text, this is a direct consequence of Eq. (IV.1), which guarantees that the two groups "forget" their original orientations and only "know" the special direction along X (i.e. along $B_\perp$), which is a common direction for the two groups.

- A property that leads to a simplification of the experimental setup is that the Rabi oscillation can be efficiently driven by MW B-field along X (i.e. the direction of $B_\perp$), enabling us to use the same coil for the pulsed field and the MW control (Fig. I.1(a)). This is also a direct consequence of Eq. (IV.1), which explicitly states that the qubit is only coupled to MW driving along X.

To see how Eq. (IV.1) generalizes to generic higher spin ($S > \frac{1}{2}$) systems, we consider the parity symmetry under the transformation $|m\rangle \leftrightarrow |-m\rangle$. Under the assumption that the zero-field Hamiltonian $H_0$ has $\pm m$ degeneracy, the perpendicular field Hamiltonian $H = H_0 + B_\perp J^x$ will be symmetric under such transformation (due to the even parity of $J^x$), leading to eigenstates with well defined and alternating parities. As an example, for NV centers used in this work, the states $|\tilde{0}\rangle$ and $|\tilde{B}\rangle$ have even parity, and the state $|D\rangle$ has odd parity. As long as we encode the qubit between a pair of eigenstates with the same parity (which are guaranteed to exist for $S > \frac{1}{2}$), we will automatically have Eq. (IV.1), because both $J^y$ and $J^z$ have odd parity under such transformation.

The above arguments show that the perpendicular field configuration is a generic method for direct tuning of the native dipolar interaction in higher spin systems, and we expect such method to find more applications beyond NV centers demonstrated in this work.


[1] P. Put, N. T. Leitao, H. Gao, C. Spaegele, O. Makarova, L. B. H. Wyatt, A. C. Maccabe, M. Mammen, B. Machielse, H. Zhou, S. Pustelny, A. C. B. Jayich, F. Capasso, L. S. Martin, H. Park, and M. D. Lukin, arXiv preprint (2025).

[2] H. Gao, L. S. Martin, L. B. Hughes, N. T. Leitao, P. Put, H. Zhou, N. U. Koyluoglu, S. A. Meynell, A. C. Jayich, H. Park, and M. D. Lukin, Nature 2025 646:8083 **646**, 68 (2025).

[3] L. S. Martin, H. Zhou, N. T. Leitao, N. Maskara, O. Makarova, H. Gao, Q. Z. Zhu, M. Park, M. Tyler, H. Park, S. Choi, and M. D. Lukin, Physical Review Letters **130**, 210403 (2023).

[4] G. Kucsko, S. Choi, J. Choi, P. C. Maurer, H. Zhou, R. Landig, H. Sumiya, S. Onoda, J. Isoya, F. Jelezko, E. Demler, N. Y. Yao, and M. D. Lukin, Physical Review Letters **121**, 023601 (2018).

[5] K. Khodjasteh and D. A. Lidar, Physical Review Letters **95**, 180501 (2005).

[6] J. Choi, H. Zhou, H. S. Knowles, R. Landig, S. Choi, and M. D. Lukin, Physical Review X **10**, 031002 (2020).

[7] T. Gullion, D. B. Baker, and M. S. Conradi, Journal of Magnetic Resonance (1969) **89**, 479 (1990).

[8] M. Tyler, H. Zhou, L. S. Martin, N. Leitao, and M. D. Lukin, Physical Review A **108**, 062602 (2023).

[9] H. Zhou, J. Choi, S. Choi, R. Landig, A. M. Douglas, J. Isoya, F. Jelezko, S. Onoda, H. Sumiya, P. Cappellaro, H. S. Knowles, H. Park, and M. D. Lukin, Physical Review X **10**, 031003 (2020).

[10] H. Zhou, L. S. Martin, M. Tyler, O. Makarova, N. Leitao, H. Park, and M. D. Lukin, Physical Review Letters **131**, 220803 (2023).

[11] J. S. Waugh, L. M. Huber, and U. Haeberlen, Physical Review Letters **20**, 180 (1968).

[12] G. A. Alvarez, A. M. Souza, and D. Suter, Physical Review A - Atomic, Molecular, and Optical Physics **85** (2012).

[13] J. J. Sakurai and J. Napolitano, *Modern Quantum Mechanics.* (Cambridge University Press, 2020).

[14] L. G. Rowan, E. L. Hahn, and W. B. Mims, Physical Review **137**, A61 (1965).
